# Supplementary material for: Budgeted and Non-budgeted Causal Bandits
Source: arXiv:2012.07058 source file (2020-12-13)
Supplement: Supplementary file 1 [file secappendix_experiments.tex]

\section{Rational for Simulation Parameters and Additional Experiments}\label{secappendix: simulations}
\subsection{Model and Parameter Choices in Section \ref{sec: experiments}}
\textbf{Experiment 1}: In this experiment the underlying causal graph and distributions $p_i = \mathbb{P}(X_i=1)$ is the same as that in \cite{LattimoreLR16}. The expected reward of the best arm is set to $0.8$ by choosing $\epsilon=0.3$. Under these settings, \cite{LattimoreLR16} demonstrated a faster exponential decay of simple regret compared to the non-causal algorithms. Since in this experiment we compare \GammaPBA to \PBA (adapted to the budgeted version), we choose the same causal graph and distribution.
%Since our baseline \PBA (in experiment $1$) is a natural extension of their algorithm, we compare our candidate \GammaPBA with \PBA using the same causal graph and distributions.

\textbf{Experiment 2}: In this experiment $2$ the underlying causal graph and distributions $p_i$ are the same as in Experiment 1. If the reward distribution is the same as in experiment $1$ the cumulative regret of \CRMPB even with $\gamma = 1.1$ converges very quickly to a small constant. This is attributed to the fact that the observation arm is closer to being optimal (i.e. $d_0$ is smaller). Even though this validates the better performance of our algorithm, for a better visual appeal we set the expected reward of the best arm to $1$. Even with this reward distribution, the performance of \CRMPB is much better than $\mathtt{F-KUBE}$.

\textbf{Experiment 3}: The causal graph used in this experiment is as shown in figure \ref{fig:generalGraph}. Notice that this graph has a backdoor path from $X_2$ to $Y$ and therefore algorithms such as \PBA, \GammaPBA and \CRMPB, which are for no-backdoor graphs, cannot be used. Our conditional probabilities for nodes ($P(\text{node}|Pa(\text{node}))$) are given in Table \ref{table: conditional distribution}.
\begin{table}[ht!]
\centering
\begin{tabular}{|l|l|}
\hline
\textbf{Conditional Variable} & \textbf{Probability} \\ \hline
$X_1=0$                       & $0.45$               \\ \hline
$X_1=1$                       & $0.55$               \\ \hline
$X_2=0 | X_1 = 0$             & $0.55$               \\ \hline
$X_2=1 | X_1 = 0$             & $0.45$               \\ \hline
$X_2=0 | X_1 = 1$             & $0.45$               \\ \hline
$X_2=1 | X_1 = 1$             & $0.55$               \\ \hline
$W_1=0 | X_1 = 0$             & $0.46$               \\ \hline
$W_1=1 | X_1 = 0$             & $0.54$               \\ \hline
$W_1=0 | X_1 = 1$             & $0.54$               \\ \hline
$W_1=1 | X_1 = 1$             & $0.46$               \\ \hline
$W_2=0 | X_2 = 0$             & $0.52$               \\ \hline
$W_2=1 | X_2 = 0$             & $0.48$               \\ \hline
$W_2=0 | X_2 = 1$             & $0.48$               \\ \hline
$W_2=1 | X_2 = 1$             & $0.52$               \\ \hline
\end{tabular}
\caption{Conditional Probability Distributions}
    \label{table: conditional distribution}
\end{table}

The conditional distribution of the reward variable $Y$ was chosen as $Y|w_1,w_2 = \theta_1 X_1 + \theta_2 X_2 + \epsilon$, where $\epsilon$ is distributed as $\mathcal{N}(0,0.01)$. Here $\mathcal{N}(0,0.01)$ denotes the normal distribution with mean $0$ and standard deviation $0.01$. Since we compare the performance of \CUCBTwo with \CUCB proposed by \cite{LU2020}, we choose our conditional distribution similar to that in \cite{LU2020}.   %where our baseline \CUCB was shown to perform better than non-causal cumulative regret minimization algorithms.
The conditional probabilities in the above table are chosen to be close to each other in order to ensure that the expected rewards for all the arms are competitive and the algorithm takes longer to distinguish between them. 
%Therefore, for the given causal graph, we will have a much fair comparison of our algorithm \CUCBTwo with the baseline \CUCB. 
The expected reward of the four arms $do(X_i = x), i\in [2], x\in \{0,1\}$ are given in the Table \ref{table: rewards}.
\begin{table}[ht!]
\centering
\begin{tabular}{|l|l|}
\hline
\textbf{Arm} & \textbf{Expected Reward} \\ \hline
$do(X_1=0)$  & $0.2595$                 \\ \hline
$do(X_1=1)$  & $0.2405$                 \\ \hline
$do(X_2=0)$  & $0.244$                  \\ \hline
$do(X_2=1)$  & $0.254$                  \\ \hline
\end{tabular}
\caption{Expected Reward of the Arms}\label{table: rewards}
\end{table}

\subsection{Additional Experiment}

In this section we show results for an additional experiment that validates our result in Theorem \ref{theorem: simple regret observational algorithm}. The experiment 4 below plots the regret of $\OBSALG$ and $\PBA$ (from \cite{LattimoreLR16}) with respect to the minimum probability. 
%$p$, and shows that the expected regret of \OBSALG decreases as $p$ increases whereas the expected regret of \PBA remains the same as $m(\mathbf{p})$ does not change.  

\textbf{Experiment $4$ ($\OBSALG $ vs.\ $\PBA$)}:
%This experiment compares the performance of $\GammaPBA$ and $\PBA$. 
This experiment demonstrates the performance of $\OBSALG$ with respect to \PBA on the same graph and parameters as chosen in Experiment $1$ of Section \ref{sec: experiments}. In figure \ref{fig:regret-vs-p-obsalg-pba}, we plot \emph{simple regret} vs. \emph{minimum probability}. Note that the minimum probability is $p = \min_{i,x}\{p_{i,x}\}$, as defined in Section \ref{subsec: obs algorithm}. We fix the budget $B$ to a moderate value $100$ and cost of intervention $\gamma$ to $1$. Note that the performance of \GammaPBA is best for $\gamma=1$. The plot shows an inverse relationship between simple regret of \OBSALG and $p$ as proved in Theorem \ref{theorem: simple regret observational algorithm}, whereas the simple regret of \PBA does not depend on $p$. Recall that the expected simple regret of \PBA depends on $m(\mathbf{p})$ (and not on $p$) and for the $p_i$'s used in Experiment $1$, the quantity $m({\bf p}) = 2$, does not change. 
%that is there are two $X_i$'s whose Bernoulli parameter is away from $\frac{1}{2}$. Since we are only changing one of these, $m({\bf p})$ still remains $2$ and the simple regret of \PBA does not depend on $p$ (as per the expression provided in Section \ref{sec: simple regret}. 
Finally, also observe that after a threshold value of $p$, \OBSALG starts performing much better than \PBA as can be seen from the plot.

\begin{figure}[ht!]
    \centering
    \includegraphics[width=60mm]{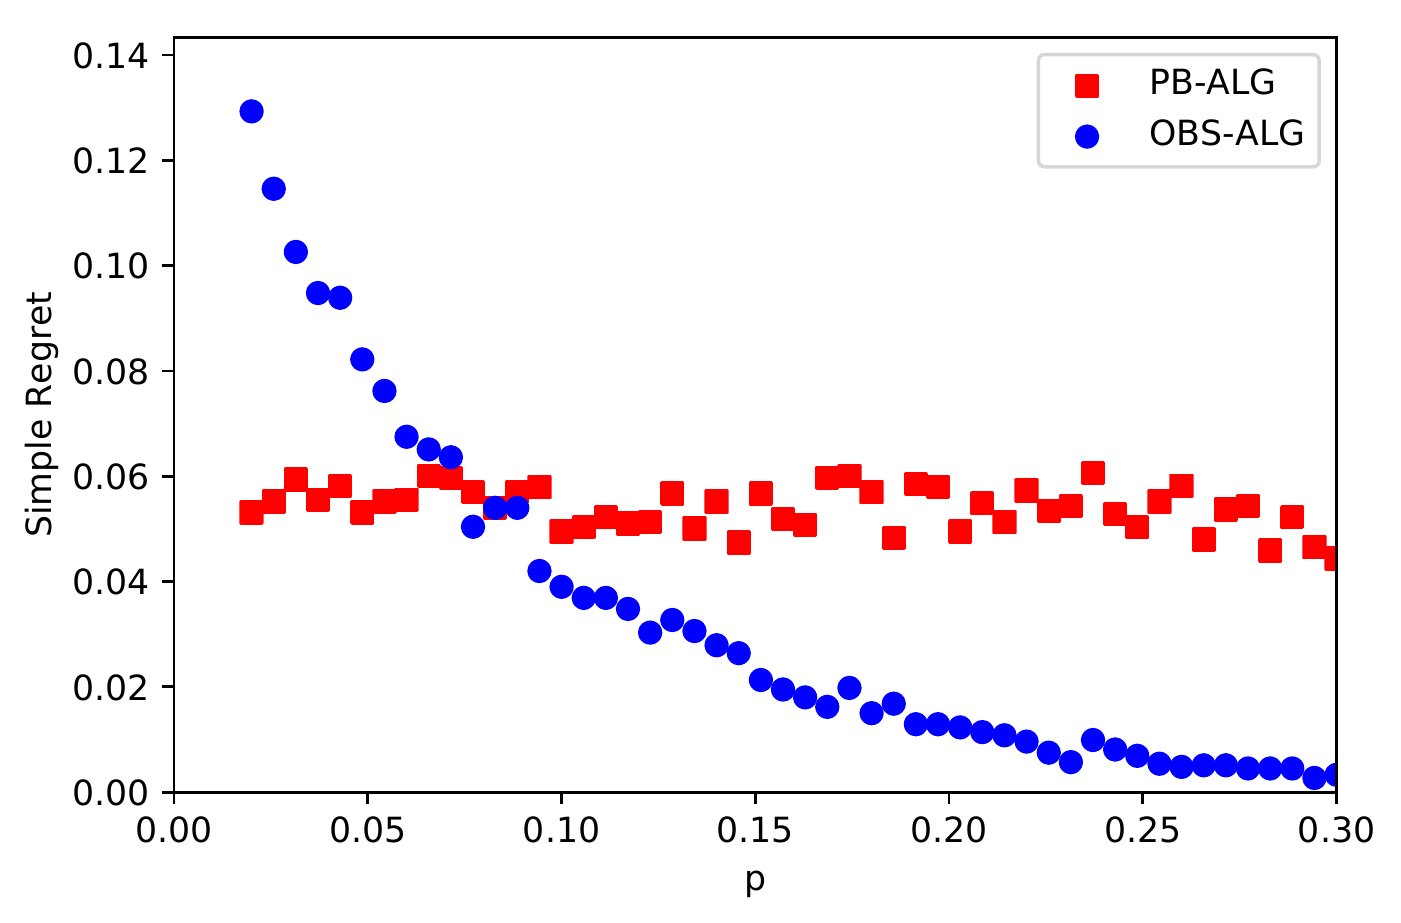}
    \caption{\OBSALG vs \PBA}
    \label{fig:regret-vs-p-obsalg-pba}
\end{figure}
